# Supplementary material for: Generative Hyperelasticity with Physics-Informed Probabilistic Diffusion Fields
Source: arXiv:2310.03745 source file (2023-09-11)
Supplement: Supplementary file 1 [file NODE_Diffusion_supplement.pdf]

# Supplement to “Generative Hyperelasticity with Physics-Informed Probabilistic Diffusion Fields”

Vahidullah Taç<sup>a</sup>, Manuel Rausch<sup>b</sup>, Ilias Bilonis<sup>a</sup>, Francisco Sahli Costabal<sup>c</sup>, Adrian Buzanza Tepole<sup>a,d</sup>

<sup>a</sup>*Department of Mechanical Engineering, Purdue University, West Lafayette, IN, USA*

<sup>b</sup>*Department of Aerospace Engineering and Engineering Mechanics, The University of Texas at Austin, Austin, TX, USA*

<sup>c</sup>*Department of Mechanical Engineering, Pontificia Universidad Catolica de Chile, Santiago, Chile*

<sup>d</sup>*Weldon School of Biomedical Engineering, Purdue University, West Lafayette, IN, USA*

## 1. Sensitivity with respect to dimensionality

Here, we vary the number of individual-specific parameters from 4 to 18 (which corresponds to increasing the width of the neural networks from 2 to 9) and compare the estimated density against the data density for the stress at  $\lambda_x = \lambda_y = 1.1$  (See Fig. 2b in the main text). To measure this mismatch, we use *energy distance* [1]. Energy distance of two distributions  $P$  and  $Q$  is defined as  $d_{\text{energy}}(P, Q) = (2\mathbb{E}|X - Y| - \mathbb{E}|X - X'| - \mathbb{E}|Y - Y'|)^{1/2}$  where the pairs  $X$  &  $X'$  and  $Y$  &  $Y'$  are independent and identically distributed random variables whose distribution is  $P$  and  $Q$ , respectively. This metric is widely used in computational science for measuring statistical proximity as it satisfies all the axioms of a distance function. As shown in Fig. 1, the training loss decreases steadily as the number of parameters is increased, meaning that the NODEs are able to better approximate the training data. However, there is minimum value for the total variation distance and it stalls at  $\approx 12$  parameters. This shows that fitting individual curves better with the NODEs comes at the expense of a worse density estimation of  $p(\phi)$  when the data is scarce.

## 2. Mixture of Gaussians for the Anisotropic case

A simple density estimation method such as mixture of Gaussians can be used to some extent in the isotropic case, where there are only a few parameters to be estimated. However, in the anisotropic case the method does a very poor job of estimating the distributions as shown in Fig. 2.

## 3. Conditioning the generative model on observed parameters

The generative model can be conditioned on an observed set of parameters  $\bar{\phi}$  shown in Fig. 3.

## 4. Convergence of the Euler-Maruyama scheme for generating heterogeneous material fields

We extended the traditional reverse SDE use in probabilistic diffusion models in order to produce heterogeneous fields of spatially correlated quantities. However, even though

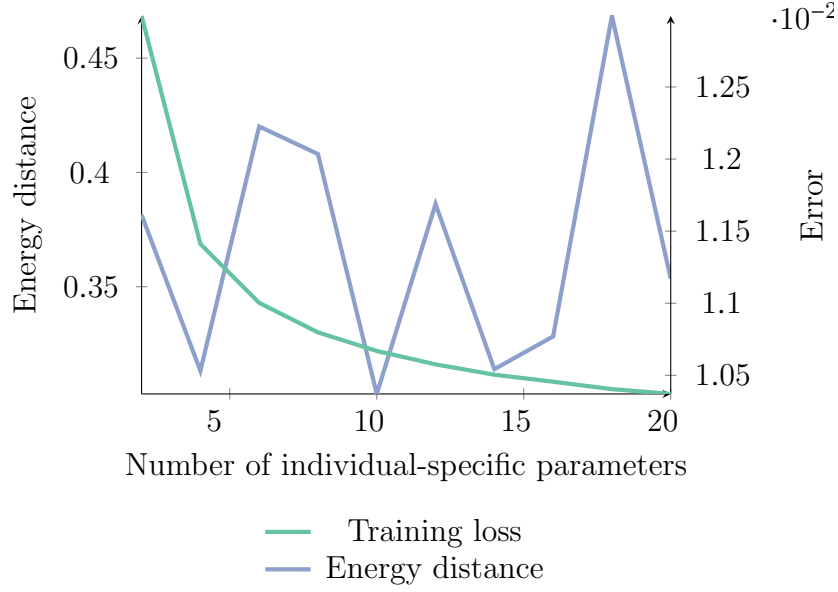

Figure 1: Sensitivity of model error and quality of density estimation with respect to the complexity of the NODE model. As the number of parameters in the NODE model increase, the stress-stretch data is fitted better (training loss decreases). The quality of the density estimation estimation is computed by determining the total variation distance between the actual distribution of a quantity of interest, e.g. stress at a given stretch, and that generated by sampling the distribution of parameters  $\hat{p}(\phi)$  using diffusion and then evaluating the NODE model to get the stress at the desired stretch.

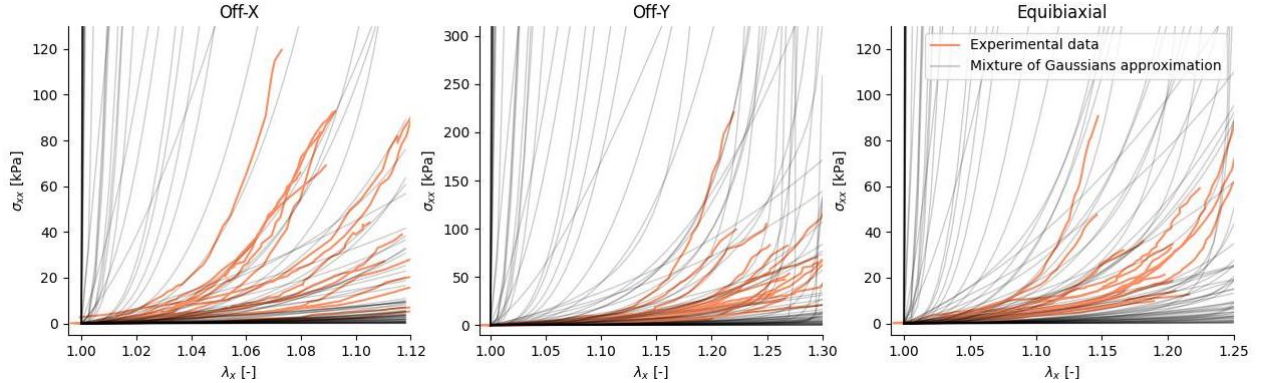

Figure 2: Performance of a mixture of Gaussians approximation in the anisotropic case. This figure shows an attempt to learn the distribution of NODE parameters with a mixture of Gaussians. The resulting stress predictions (gray) are not indicative of the training population (orange).

the traditional reverse SDE is well-defined and should converge with the Euler-Maruyama scheme, the same is not true when considering samples from GPs which are advanced in time with the addition of spatially correlated noise in the form of additional GP samples. Fig. 4 shows that the Euler-Maruyama scheme for the spatial stochastic process indeed converges with respect to the number of samples, the resolution of the spatial sampling, and the time step.

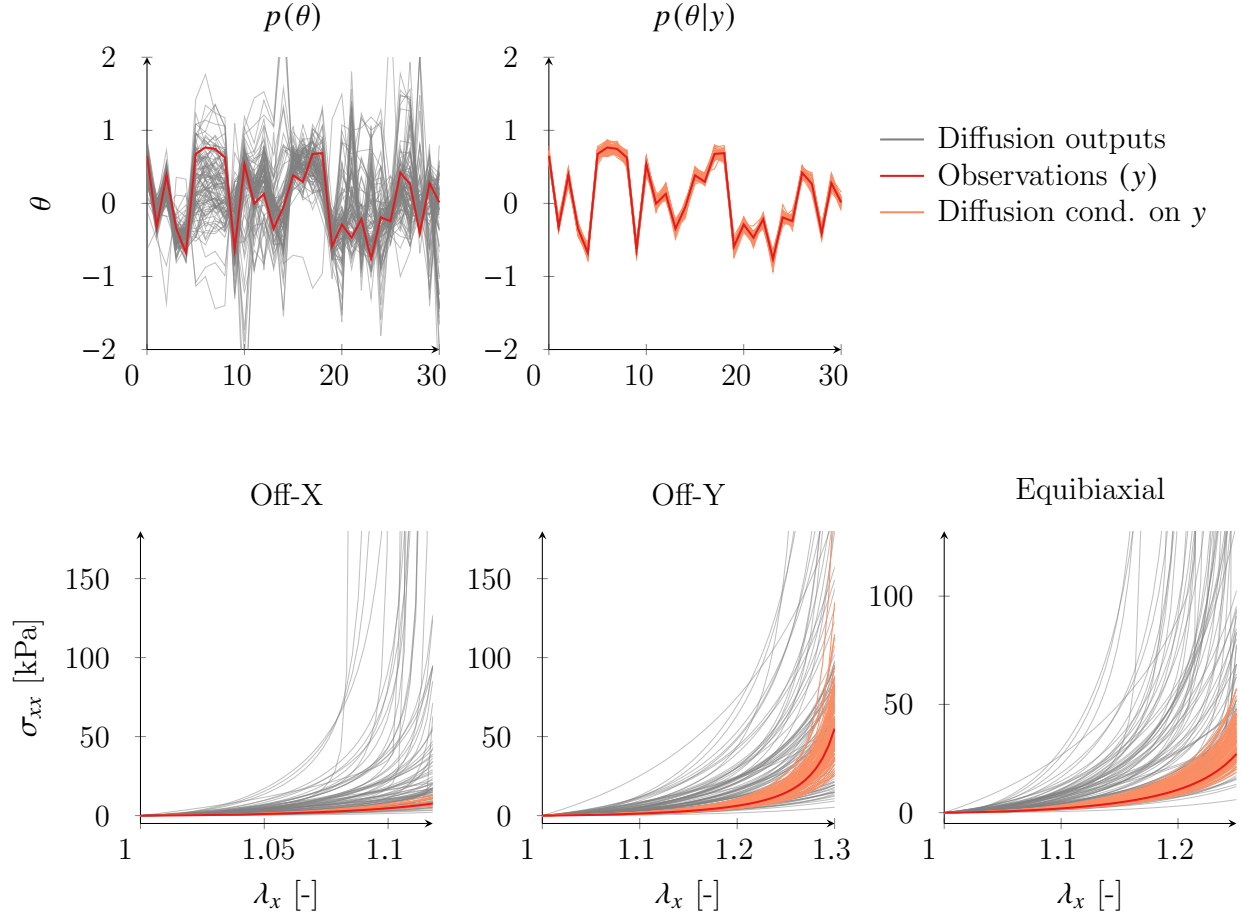

Figure 3: Conditioning the generative process on observing parameters  $\bar{\phi}$  with some variance  $\varsigma$ .

## References

- [1] M. L. Rizzo, G. J. Székely, Energy distance, Wiley Interdisciplinary Reviews: Computational Statistics 8 (1) (2016) 27–38. doi:10.1002/wics.1375.

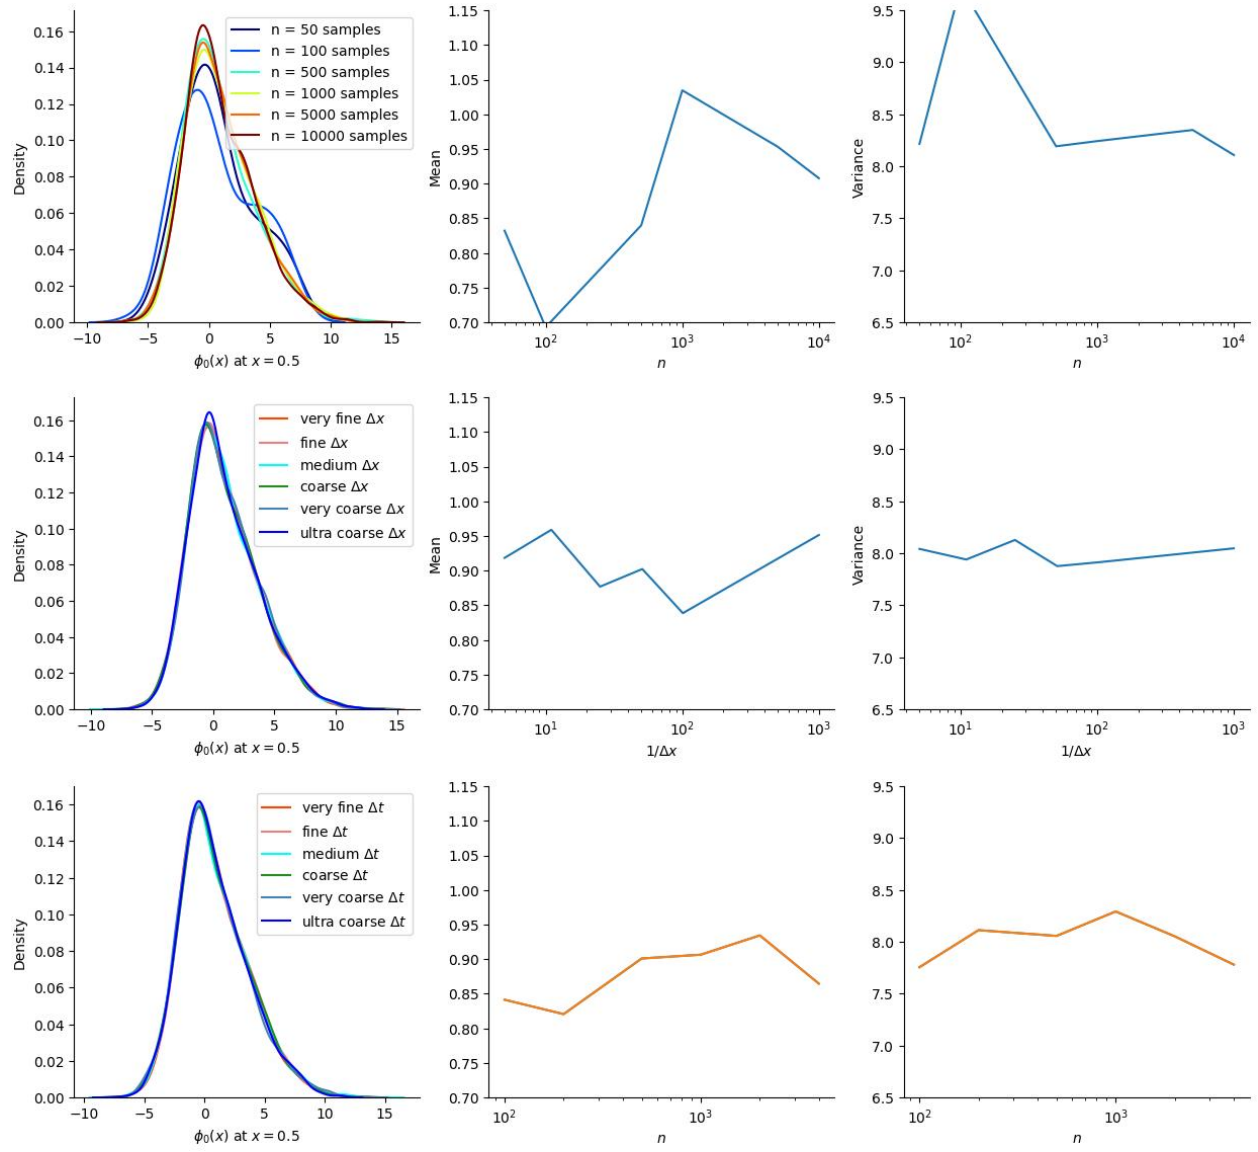

Figure 4: Convergence of the Euler-Maruyama scheme for different sample sizes (top row), spatial discretization (middle row) and time step sizes (bottom row).
